# Supplementary material for: SHADOWCAST: Controllable Graph Generation
Source: arXiv:2006.03774 source file (2021-07-02)
Supplement: Supplementary file 1 [file appendix.tex]

\section*{Appendix}
% ================ section ================
\subsection*{A. Implementation Details}
% \subsection*{A.1: Implementation Details}

The \textsc{ShadowCast} model incorporates a sequence-to-sequence (Seq2Seq) learner, a generator, and a discriminator.

\paragraph{Shadow Caster (Seq2Seq)}
In the sequence-to-sequence model, we use an LSTM with 10 cells for all three datasets. The input of this LSTM is a batch of shadow walk sequences length n and dimension d, where the batch size is 128, walk length 16, and dimension is set as the number of classes $K$ in each dataset (128 x 16 x d). We select the walk length as 16 because it should capture structures of most graphs of different sizes. The LSTM hidden layer with 10 memory units should be more than sufficient to learn this problem. A dense layer with Softmax activation is connected to the LSTM layer, and the generated output is a batch of sequences with size (128 x 16 x d).

\paragraph{Generator}
In the generator, we use a conditional LSTM with 50 layers. We follow a similar architecture to NetGAN to generate sequences of walks on the graph nodes. Different from NetGAN, our generator not only initializes the model with Gaussian noise, but it also takes the shadow walks as conditions at each step of the process. Interestingly, we notice that the LSTM generator is more sensitive to the input conditions than hyperparameters for performance. Hence, the set of hyperparameters for the generator is the same for all the datasets. We summarize the generative process of $G$ below. We note that the conditional generative process is similar to the unconditional process of NetGAN, with the addition of conditions $\tilde{\bm{s}}_t$ in each timestep.

\begin{figure}[htbp] 
\centering 
\begin{adjustbox}{minipage=\linewidth,scale=0.75}
\begin{empheq}{align*}%[box=\fbox]{align*}
    &  &\bm{\bm{z}} \sim & \ \mathcal{N}(\bm{0}, \bm{I}_d) & & \\
    &t=0  &\bm{m}_0 &= g_{\theta'}(\bm{\bm{z}}) & & \\
    % \bm{s}_0 &= \bm{0} & & &\\
    &t=1  &f_\theta(\bm{m}_0, \tilde{\bm{s}}_1, \bm{0}) &= (\bm{p}_1, \bm{m}_1),  & \bm{v}_1 &\sim Cat(\sigma(\bm{p}_1)) \\
    &t=2  &f_\theta(\bm{m}_1, \tilde{\bm{s}}_2, \bm{v}_1) &= (\bm{p}_2, \bm{m}_2),  & \bm{v}_2 & \sim Cat(\sigma(\bm{p}_2)) \\
    &\quad\vdots  & &\ \ \vdots & & \qquad \vdots \\
    &t=T  &f_\theta(\bm{m}_{T-1}, \tilde{\bm{s}}_{T}, \bm{v}_{T-1}) &= (\bm{p}_T, \bm{m}_T),  & \bm{v}_T & \sim Cat(\sigma(\bm{p}_T)) 
\end{empheq}
\end{adjustbox}
\end{figure}

\paragraph{Discriminator}
Our discriminator is an LSTM with 40 layers. The inputs are sequences of graph nodes concatenated with the respective conditions. The discriminator has similar architecture as the shadow caster, where they are LSTM models that take sequences as inputs, expect that the LSTM layer is connected to a final dense layer. The output is a single value between 0 and 1, which distinguishes real sequences from generated ones.

In the \textsc{ShadowCast} training, we use Adam optimizers for all the models. The learning rate of the shadow caster sequence-to-sequence training is 0.01, while both the generator and the discriminator use a learning rate of 0.0002.

% ================ section ================
% \section*{APPENDIX B: Baselines}
\subsection*{B. Baselines}

\begin{itemize}
    \item \textbf{CondGEN.} We use the official PyTorch implementation (\url{https://github.com/KelestZ/CondGen}). However, CondGEN is designed to learn a distribution over multiple small graphs. To ensure a fair comparison, we modify it to train on randomly selected $85\%$ of the edges in a graph, validate on the remaining $15\%$, and generate graphs. 
    
    \item \textbf{GraphRNN.} We use the official PyTorch implementation (\url{https://github.com/JiaxuanYou/graph-generation}) of GraphRNN. The default hyperparameter settings were used in all our experiments. 
    
    \item \textbf{GVAE.} To compare with Graph VAE (no public code available), we adapt the reference implementation provided by~\citet{NIPS2019_8415} in their experiments for a single graph and use the suggested hyperparameter settings. 
    
    \item \textbf{NetGAN.} We use the official TensorFlow implementation provided by the authors (\url{https://github.com/danielzuegner/netgan}), following the recommended hyperparameter settings. We set \texttt{random walk length} to 16, \texttt{learning rate} to 0.0003, \texttt{generator L2 penalty} to 1e-7, and \texttt{discriminator L2 penalty} to 5e-5.    
\end{itemize}

% ================ section ================    
% \section*{APPENDIX C: Datasets}
\subsection*{C. Datasets}

Details of the datasets are listed below (see \cref{table:datasets}).

\begin{table}[htbp]
\centering
\resizebox{.95\linewidth}{!}{%
\begin{tabular}{
    >{\centering\arraybackslash}m{3cm}% instead of "p" is "m"
    |>{\centering\arraybackslash}m{1.5cm}
    >{\centering\arraybackslash}m{1.5cm}
    >{\centering\arraybackslash}m{1.5cm}
    >{\centering\arraybackslash}m{3cm}
    }
    \textbf{Dataset} & \textbf{N$_{LCC}$} & \textbf{E$_{LCC}$} & \textbf{K classes} & \textbf{K distribution} \\ \hline \hline 
    \textit{Cora-ML} &2810 &7981 &7 &\vspace{.5mm}\includegraphics[width=.2\textwidth]{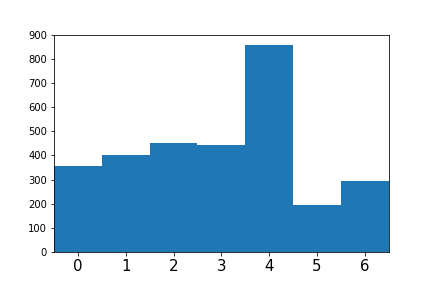} \\ \hline 
    \textit{Enron} &154 &1843 &3 &\vspace{.5mm}\includegraphics[width=.2\textwidth]{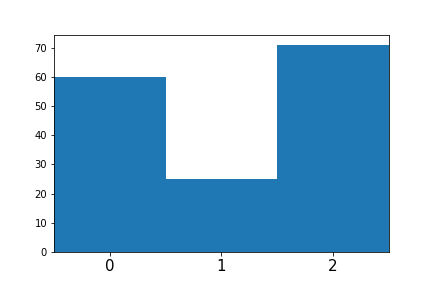} \\ \hline 
    \textit{EUcore-top} &348 &3342 &5 &\vspace{.5mm}\includegraphics[width=.2\textwidth]{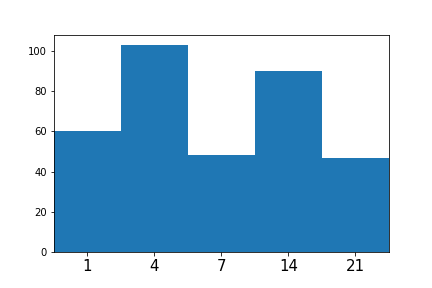}   \\     
\end{tabular}}
\caption{Statistics of datasets. In the largest connected component (LCC) of each dataset, N$_{LCC}$ is the number of nodes, E$_{LCC}$ the edges, and K number of total classes. The distribution of the classes is shown in the corresponding histograms. \label{table:datasets}}
\end{table}

\begin{itemize}
    \item \textit{EUcore-top}: An email communication network we created that consists of the top five largest departments in the EU-core dataset~\citep{leskovec2007graph}. For all nodes in the graph, if a person $i$ sends at least one email to person $j$, then there exists an edge $(i,j)$ between the two nodes. Each node belongs to exactly one department. We sort the data by the intra-department email counts in descending order. The list of top five departments is $\{14, 4, 7, 21, 1\}$. Link here: \url{http://snap.stanford.edu/data/email-Eu-core.html}
    
    \item \textit{Enron}: It is the Enron Corporation email corpus dataset~\citep{Perry_2013}, where an edge exists between any two nodes as long as they share at least one email. Link here: \url{https://github.com/patperry/interaction-proc/tree/master/data/enron}
    
    \item \textit{Cora-ML}: A scientific publication citation dataset~\citep{bojchevski2018deep} consisting of machine learning papers. Link here: \url{https://github.com/abojchevski/graph2gauss/tree/master/data}
\end{itemize}

\subsection*{D. Controlling Generated Graphs}

We provide the Markov model parameters, initial probability distribution $\bm{\pi} = (\pi_1, \pi_2, \pi_3)$ and transition probability matrix $\bm{A} = (a_{11}a_{12}\dots a_{31}\dots a_{33})$, used in our experiments.

\begin{figure}[htbp]
    \centering
    \includegraphics[width=.9\linewidth]{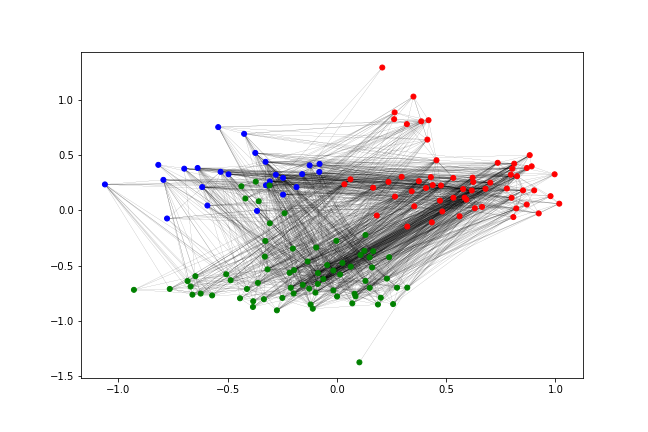}
    \caption*{\textbf{Observed:} \textit{Enron} normal operations}
    % \label{fig:ShadowCast_architecture}
\end{figure}

% G_control1 = controlled_generation(init_distr=[0.9, .05, .05], 
%                                   transitionMatrix=[[0.9,0.05,0.05],[0.1,0.6,0.3],[0.0,0.1,0.9]], 
%                                   multiplier=1, controlgen_iter=100, control_dept_list=dept_list, 
%                                   condition_dim=n_conds, rw_len=4)
\begin{figure}[htbp]
    \centering
    \includegraphics[width=.9\linewidth]{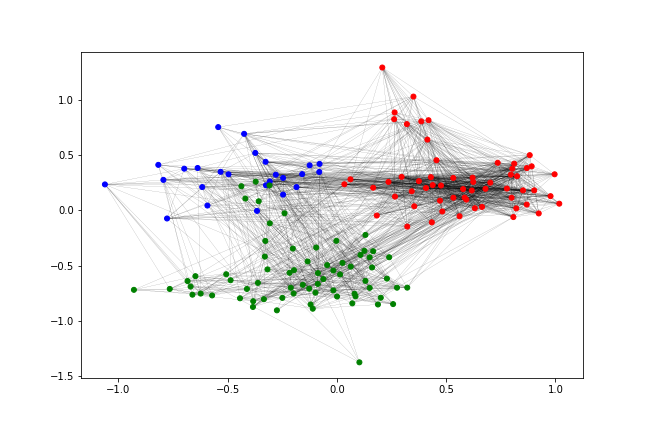}
    \caption*{\textbf{Generated:} Legal (red) internal surge \\
    \textbf{Initial probability distribution:} \\ $\bm{\pi} = [0.9, 0.05, 0.05]$ \\
    \textbf{Transition probability matrix:} \\ $\bm{A} = [[0.9,0.05,0.05],[0.1,0.6,0.3],[0.0,0.1,0.9]]$}
    % \label{fig:ShadowCast_architecture}
\end{figure}

% G_control2 = controlled_generation(init_distr=[0.05, .05, .9], 
%                                   transitionMatrix=[[0.9,0.1,0.0],[0.1,0.6,0.3],[0.05,0.05,0.9]], 
%                                   multiplier=1, controlgen_iter=100, control_dept_list=dept_list, 
%                                   condition_dim=n_conds, rw_len=4)
\begin{figure}[htbp]
    \centering
    \includegraphics[width=.9\linewidth]{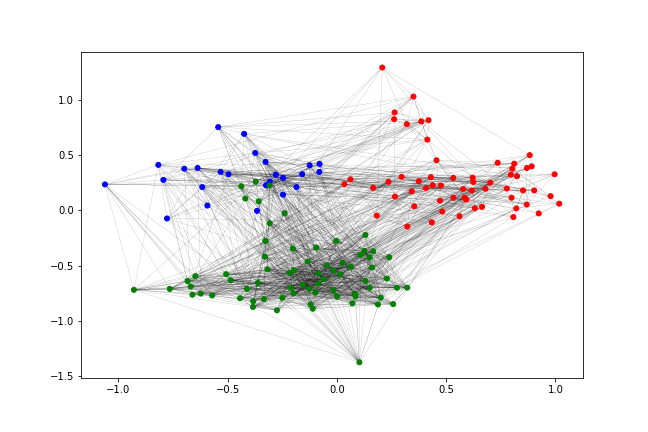}
    \caption*{\textbf{Generated:} Finance (green) internal surge \\
    \textbf{Initial probability distribution:} \\ $\bm{\pi} = [0.05, 0.05, 0.9]$ \\
    \textbf{Transition probability matrix:} \\ $\bm{A} = [[0.9,0.1,0.0],[0.1,0.6,0.3],[0.05,0.05,0.9]]$} 
    % \label{fig:ShadowCast_architecture}
\end{figure}

% G_control3 = controlled_generation(init_distr=[0.05, .9, .05], 
%                                   transitionMatrix=[[0.9,0.1,0.0],[0.25,0.5,0.25],[0.0,0.1,0.9]],
%                                   multiplier=1, controlgen_iter=100, control_dept_list=dept_list, 
%                                   condition_dim=n_conds, rw_len=4)
\begin{figure}[htbp]
    \centering
    \includegraphics[width=.9\linewidth]{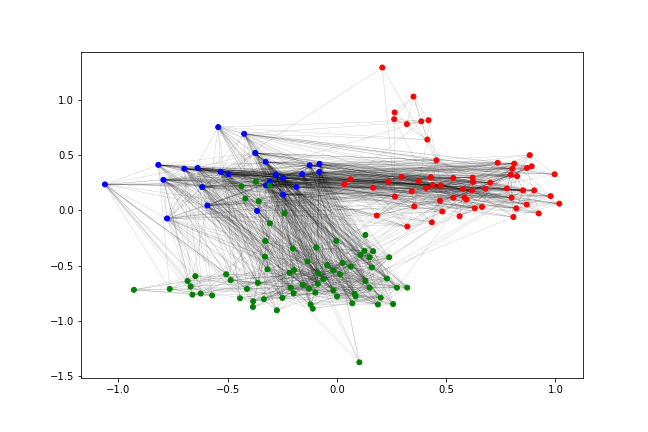}
    \caption*{\textbf{Generated:} Trading (blue) outgoing surge \\
    \textbf{Initial probability distribution:} \\ $\bm{\pi} = [0.05, 0.9, 0.05]$ \\
    \textbf{Transition probability matrix:} \\ $\bm{A} = [[0.9,0.1,0.0],[0.25,0.5,0.25],[0.0,0.1,0.9]]$} 
    % \label{fig:ShadowCast_architecture}
\end{figure}
